# Supplementary material for: NashFormer: Leveraging Local Nash Equilibria for Semantically Diverse Trajectory Prediction
Source: arXiv:2305.17600 source file (2023-11-11)
Supplement: Supplementary file 1 [file additional_qualitative.tex]

\subsection{Additional Qualitative Results}

We present additional qualitative results on the next page.

\begin{figure}[h!]
\centering
    \begin{tabular}{ccc}
        \subfigure[Agent $2$ may choose to divert its route depending on when agent $1$ turns.]{\includegraphics[width=0.32\linewidth]{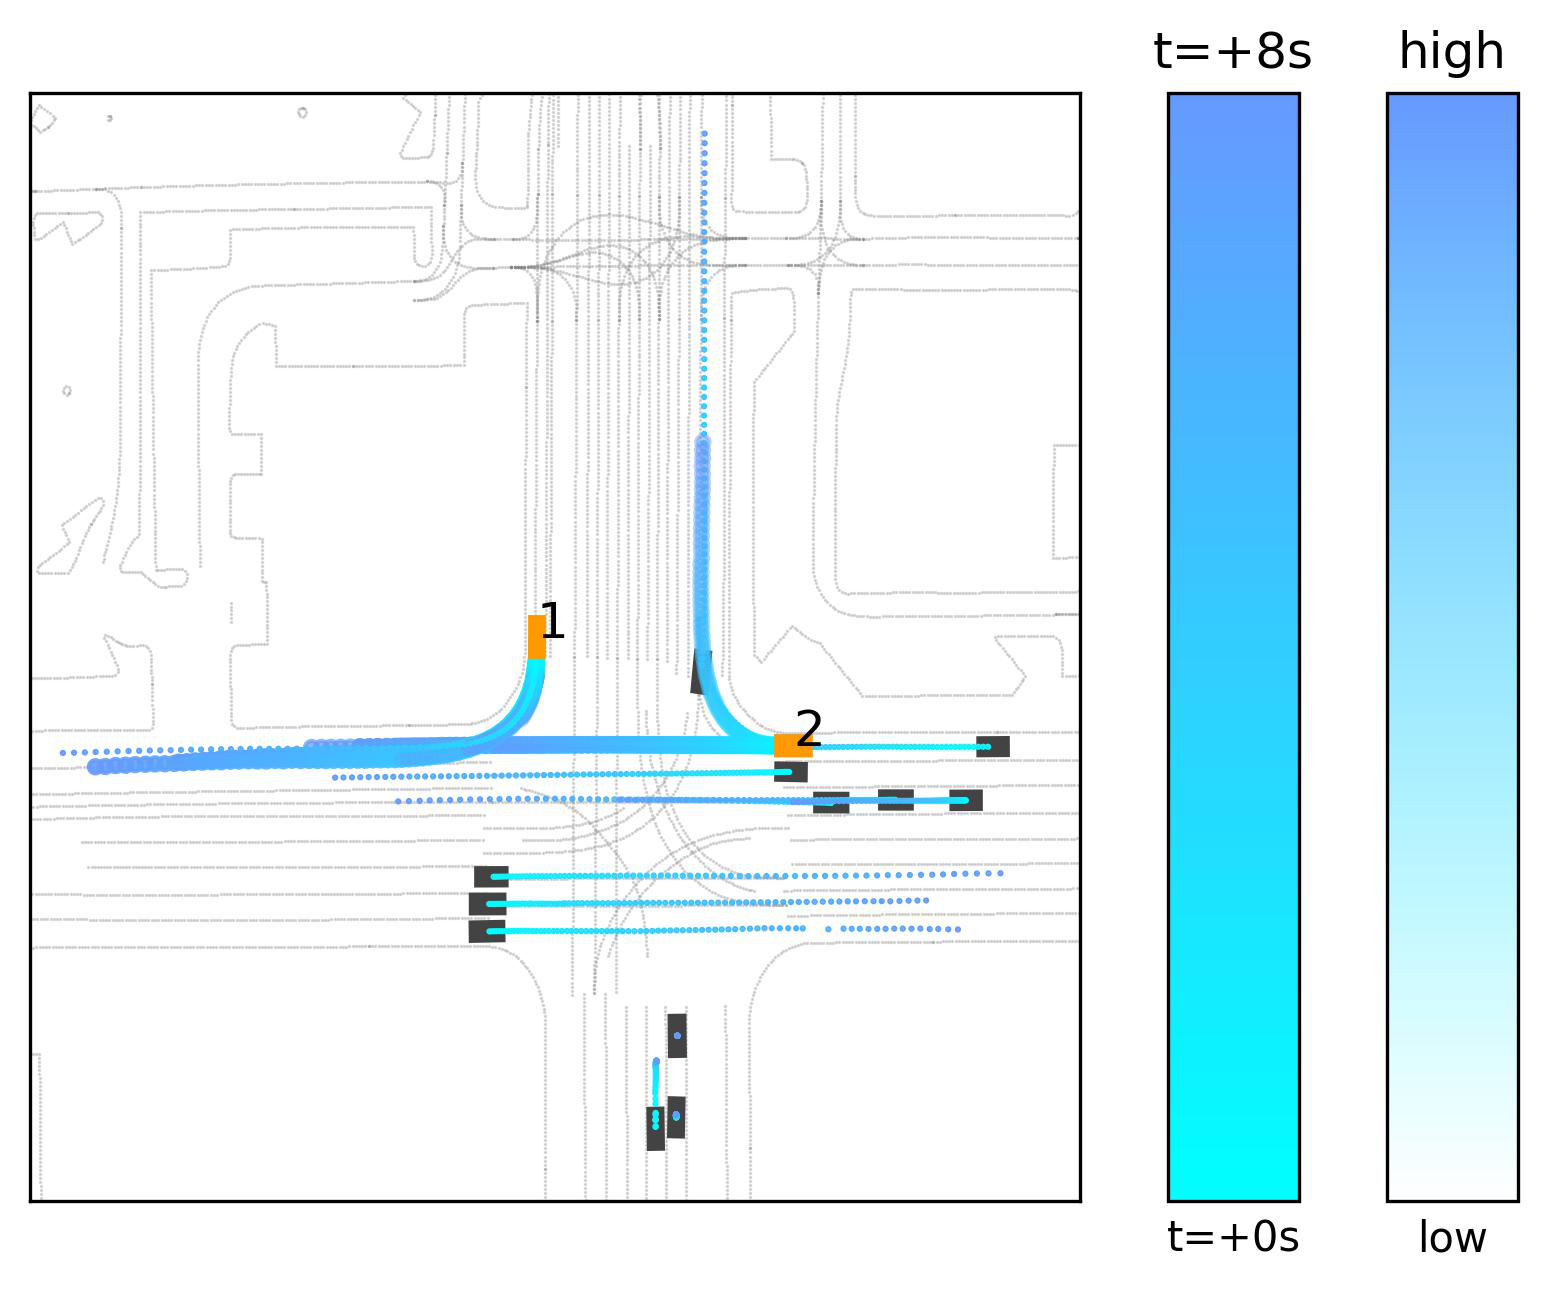}} &
        \subfigure[Agent $1$ may perform a pass of the slower agent $2$ with various degrees of aggression.]{\includegraphics[width=0.32\linewidth]{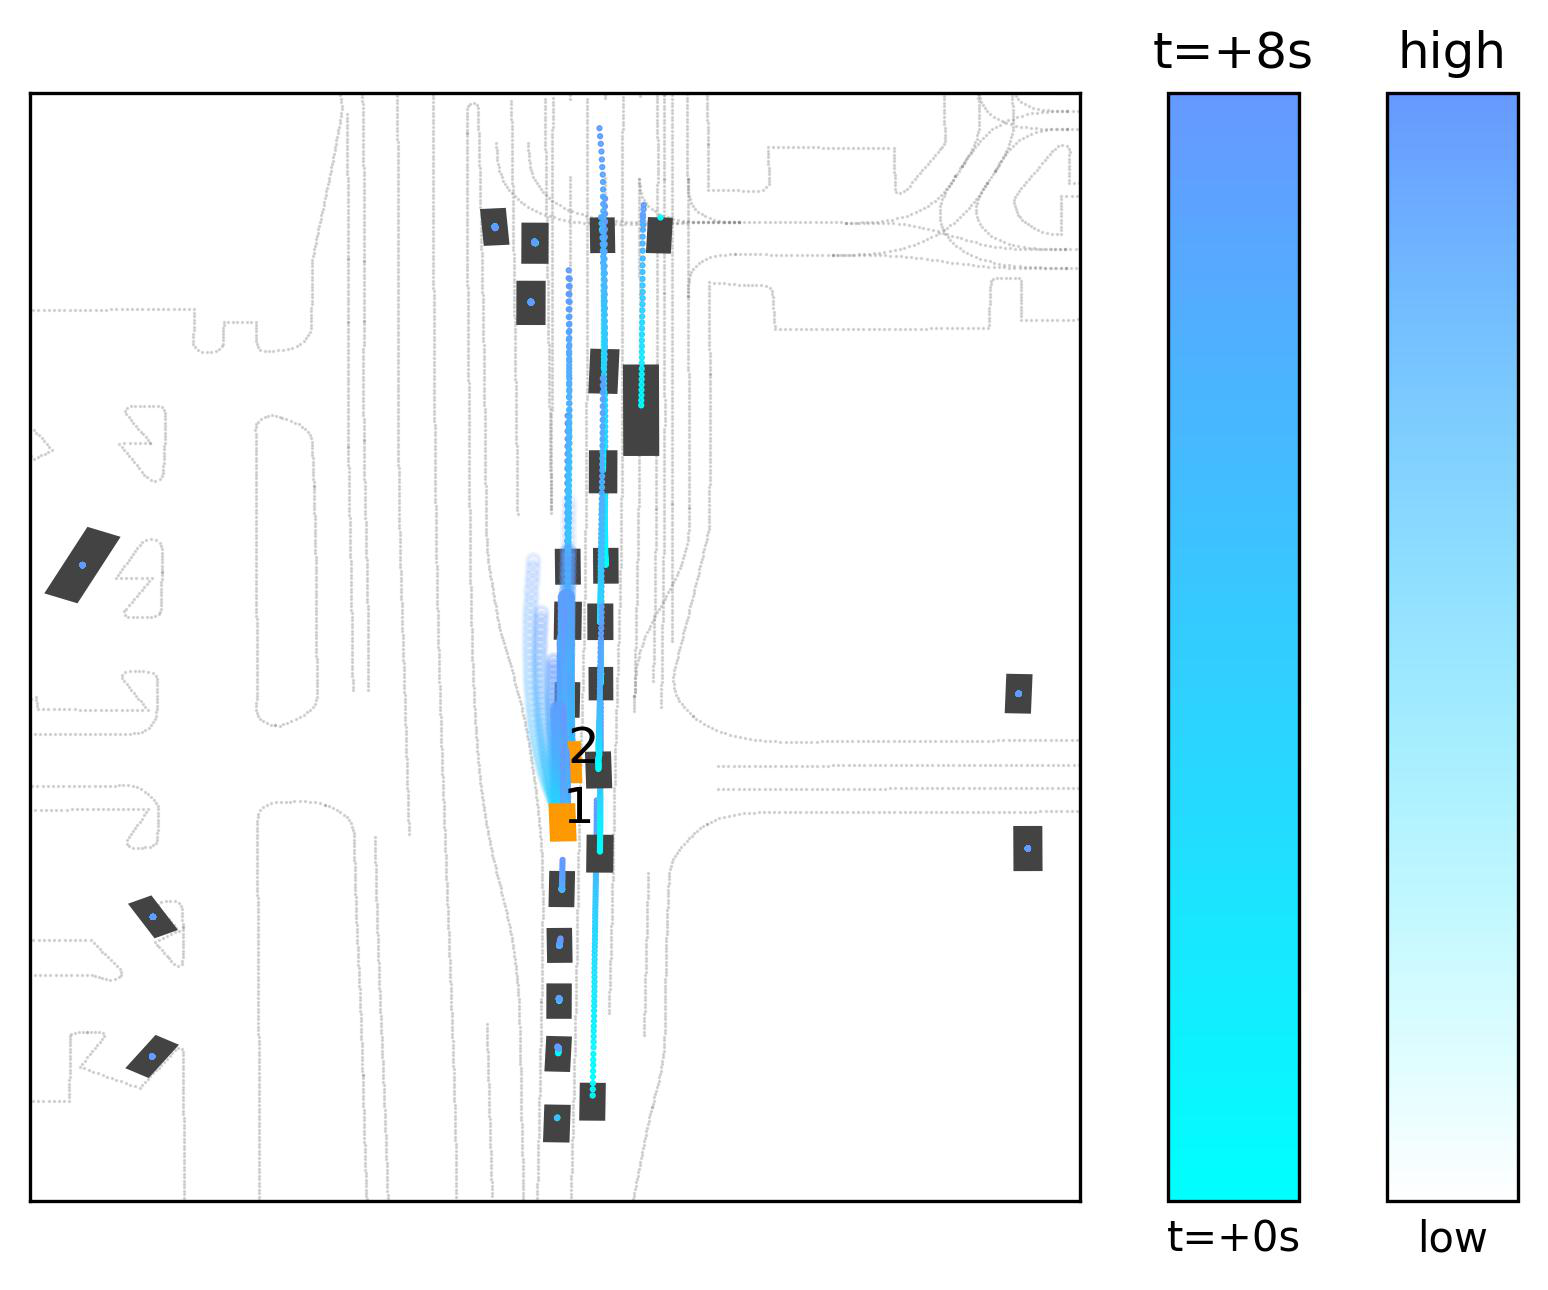}} & 
        \subfigure[Agent $2$ unexpectedly cuts off agent $1$, who is a pedestrian with right-of-way, resulting in an extreme, but anticipated, yield exchange. ]{\includegraphics[width=0.32\linewidth]{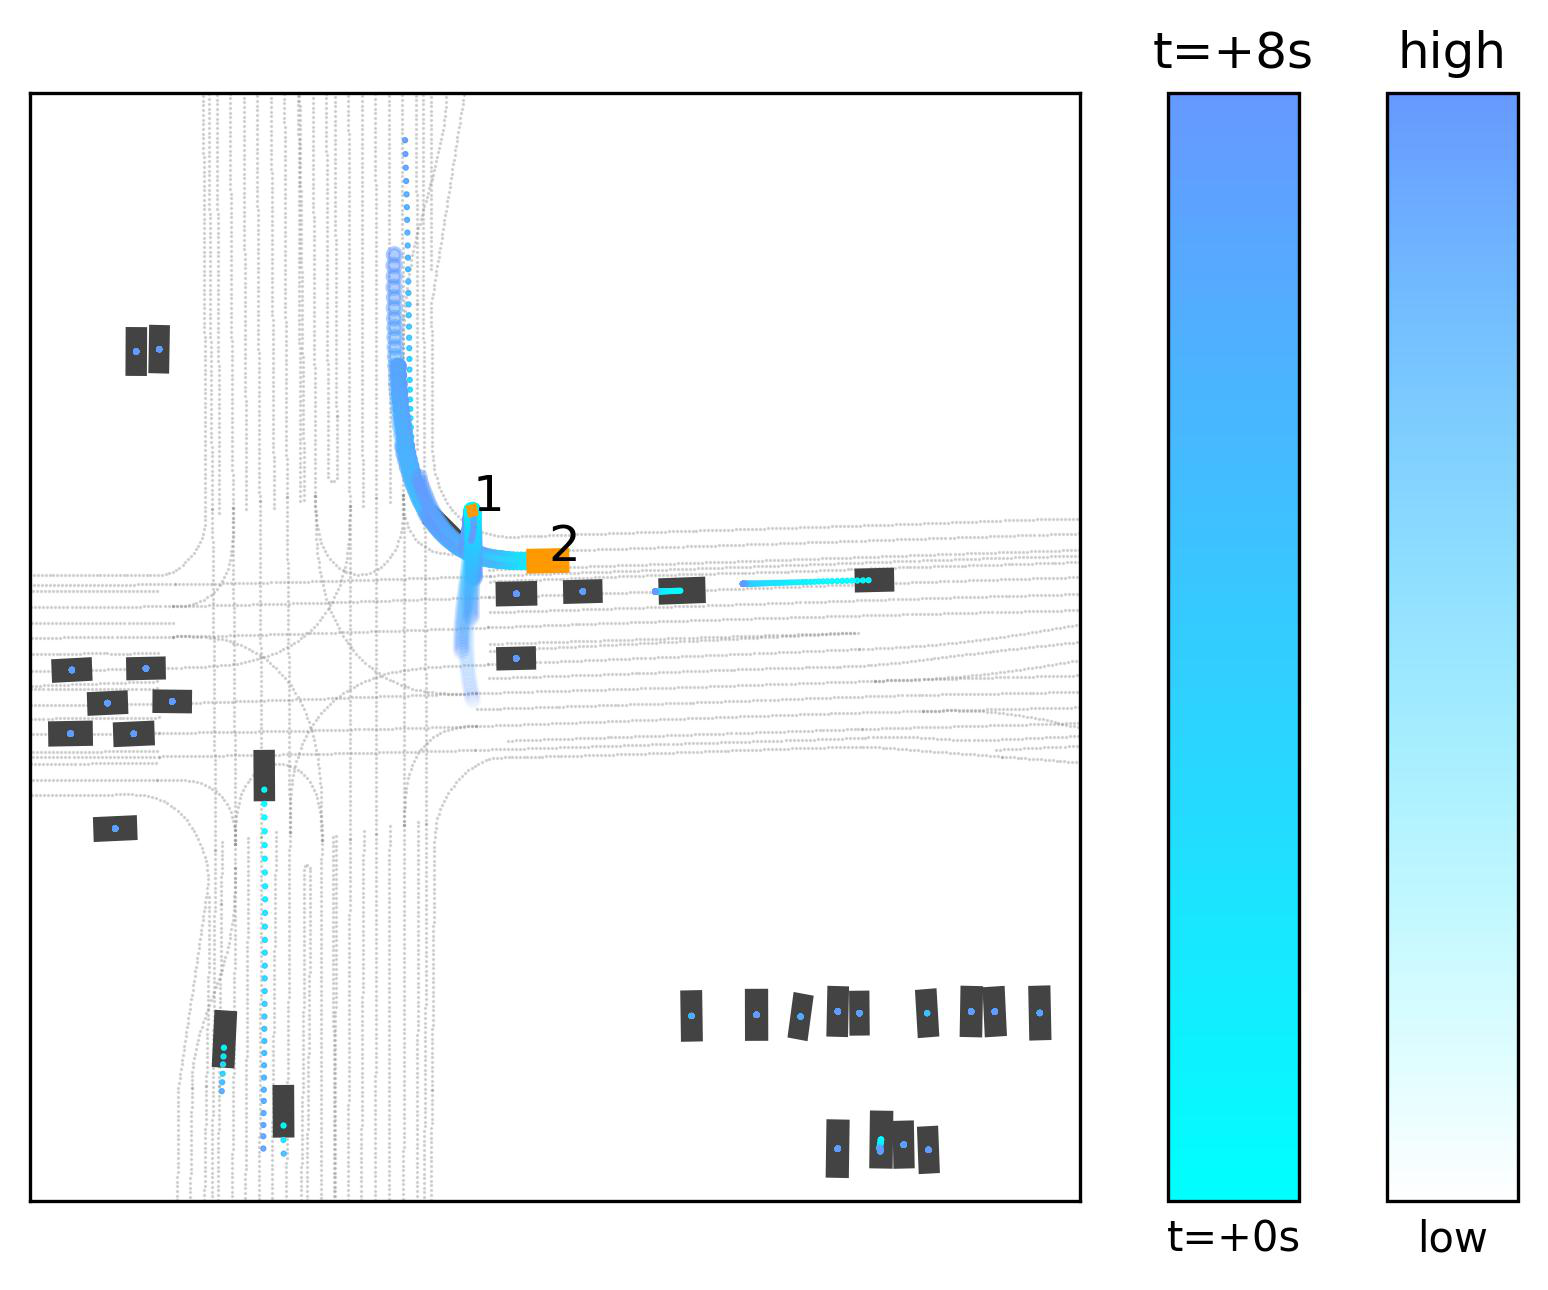}} \\ 
        \subfigure[Agent $2$ must time their turn depending on agent $1$'s choice, either to turn or go straight. Agent $2$ must anticipate both a slower and faster agent $1$. ]{\includegraphics[width=0.32\linewidth]{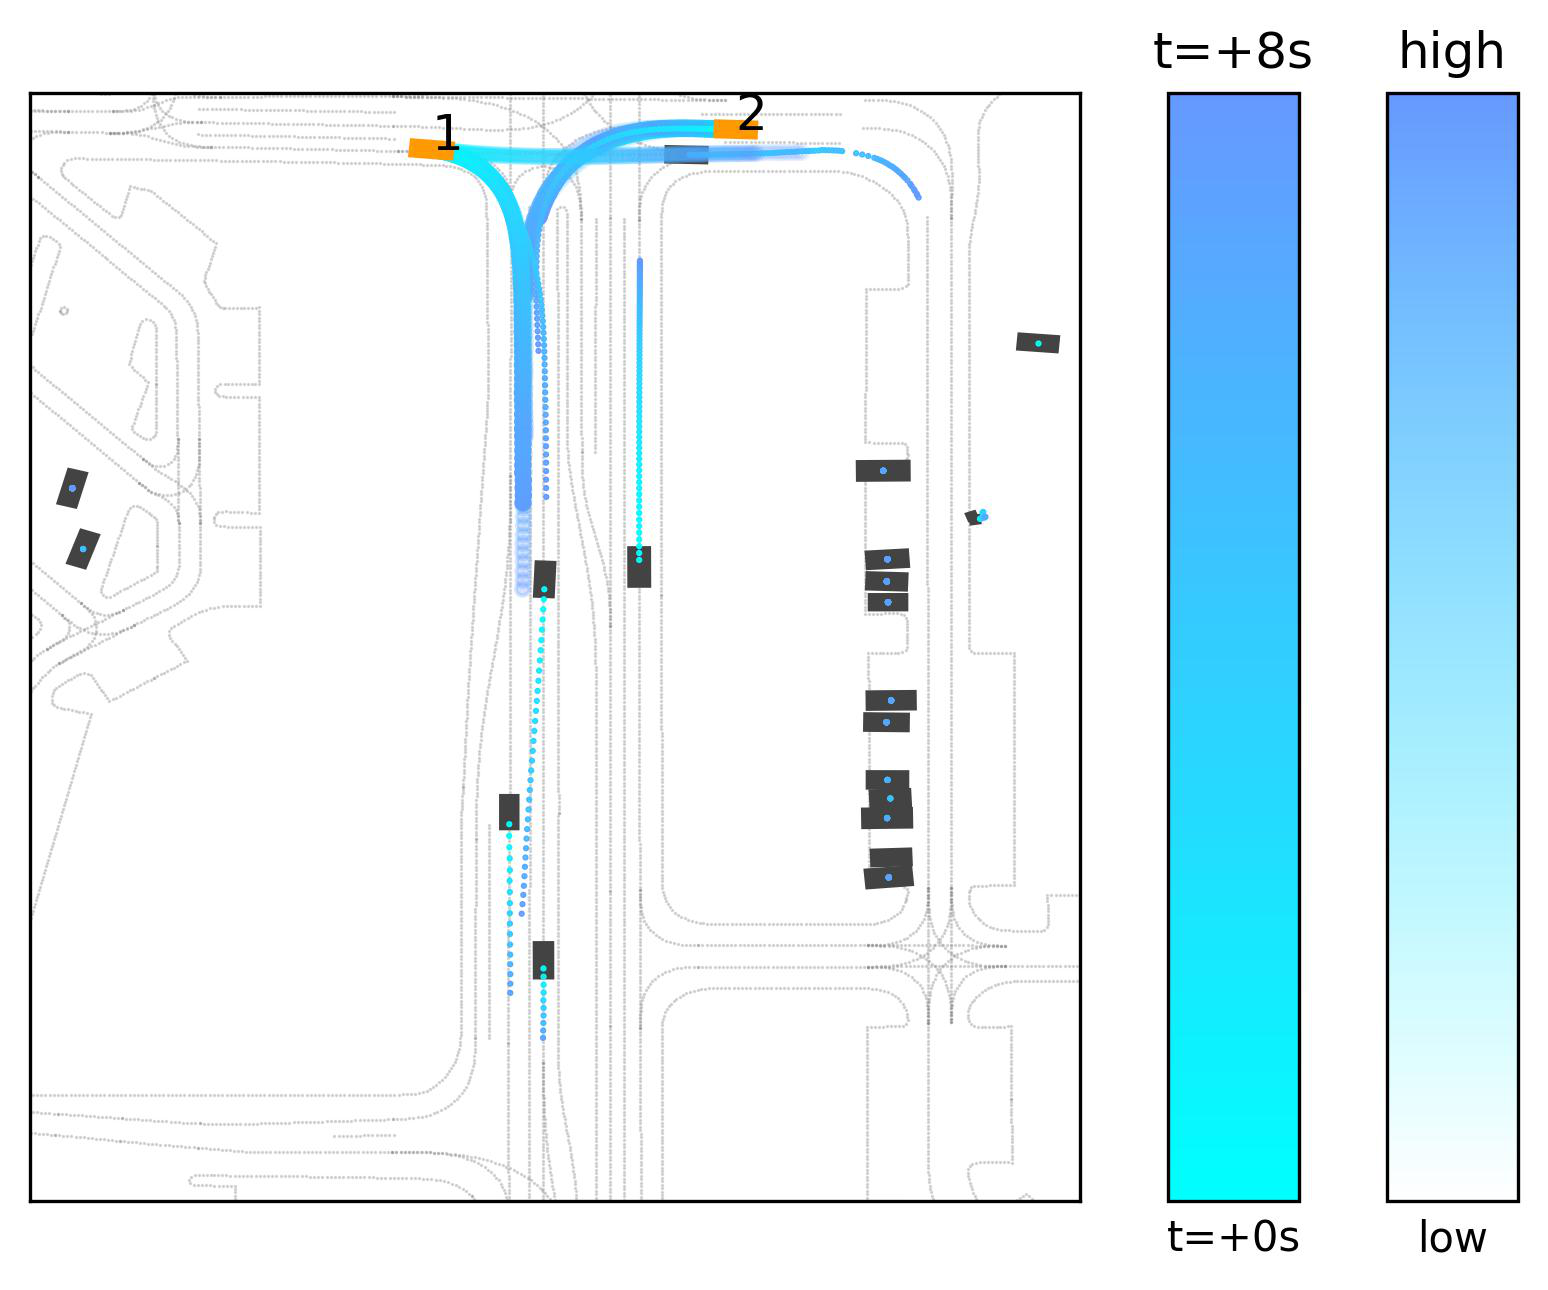}} &
        \subfigure[Agent $2$ may turn abruptly, possibly interrupting agent $1$'s expected course. Agent $1$ anticipates both exchanges.]{\includegraphics[width=0.32\linewidth]{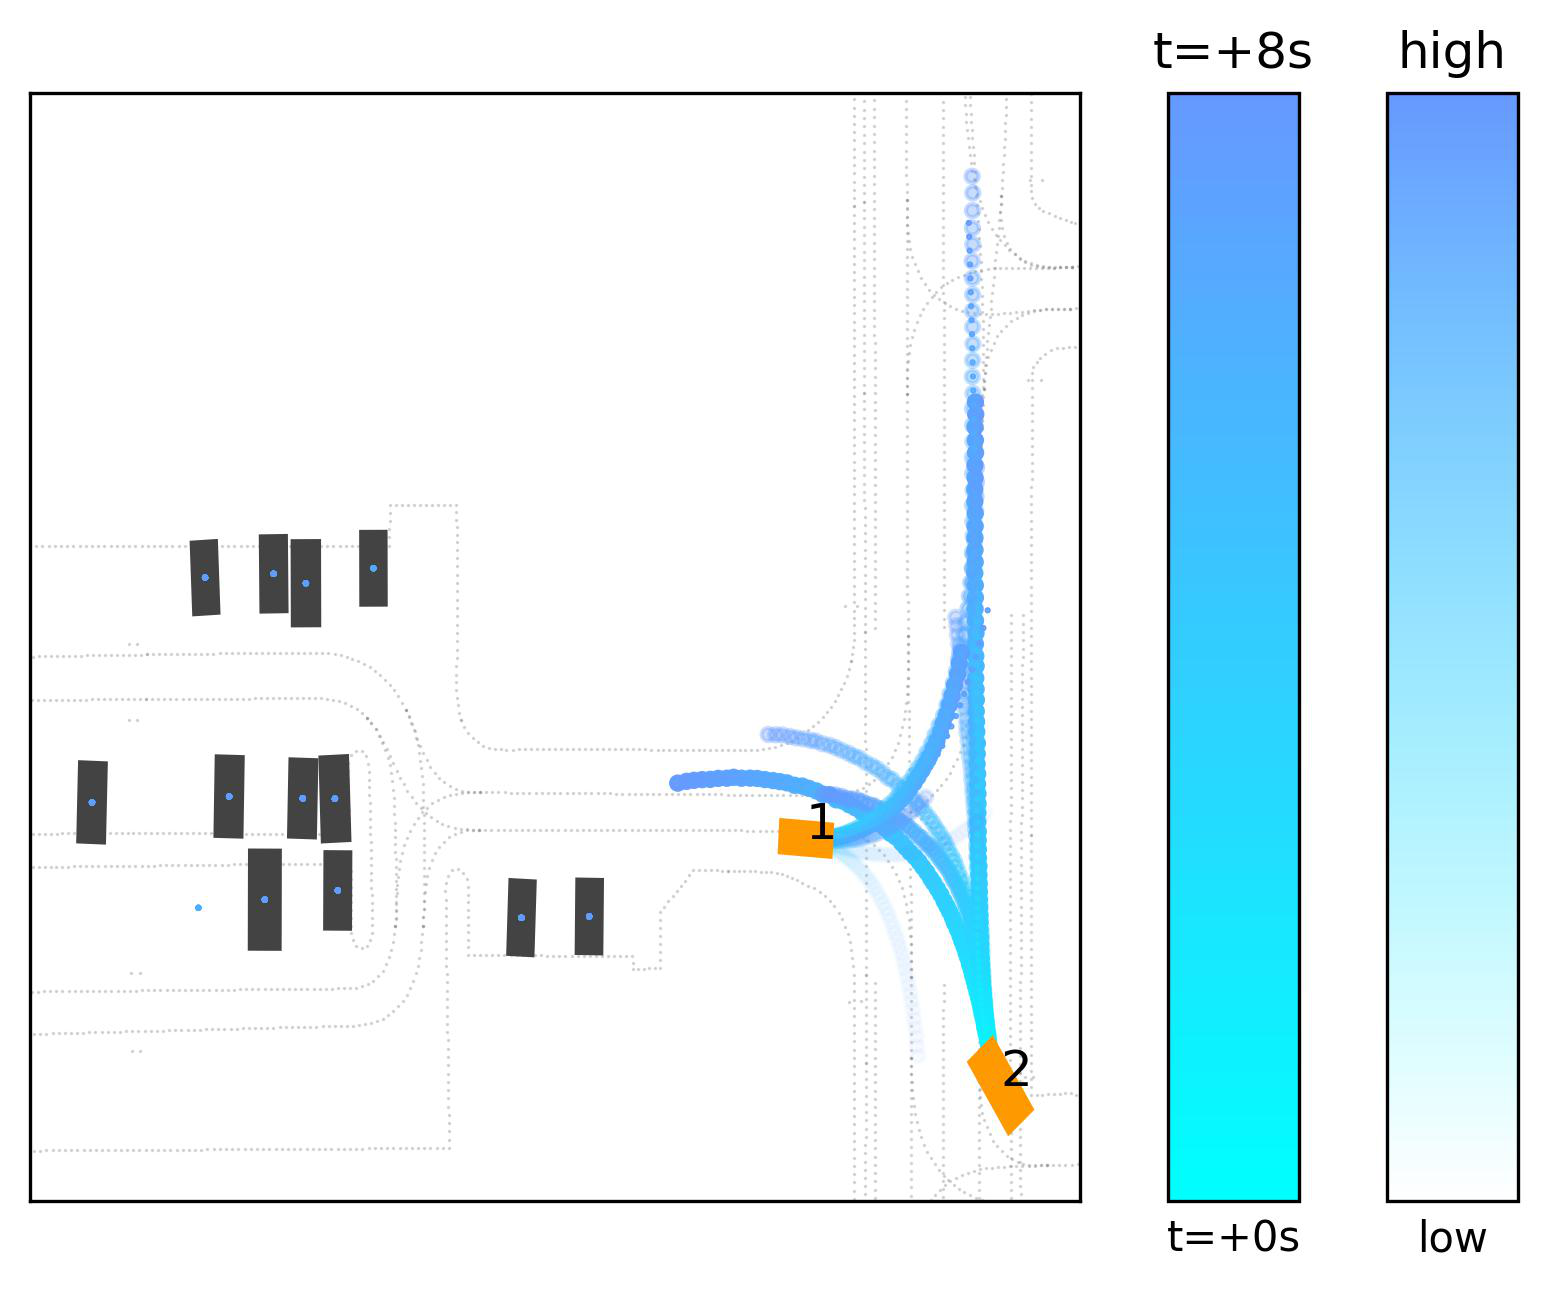}} & 
        \subfigure[Agent $1$ is expected to rapidly turn left into traffic, affecting the timing of agent $2$'s maneuvers. ]{\includegraphics[width=0.32\linewidth]{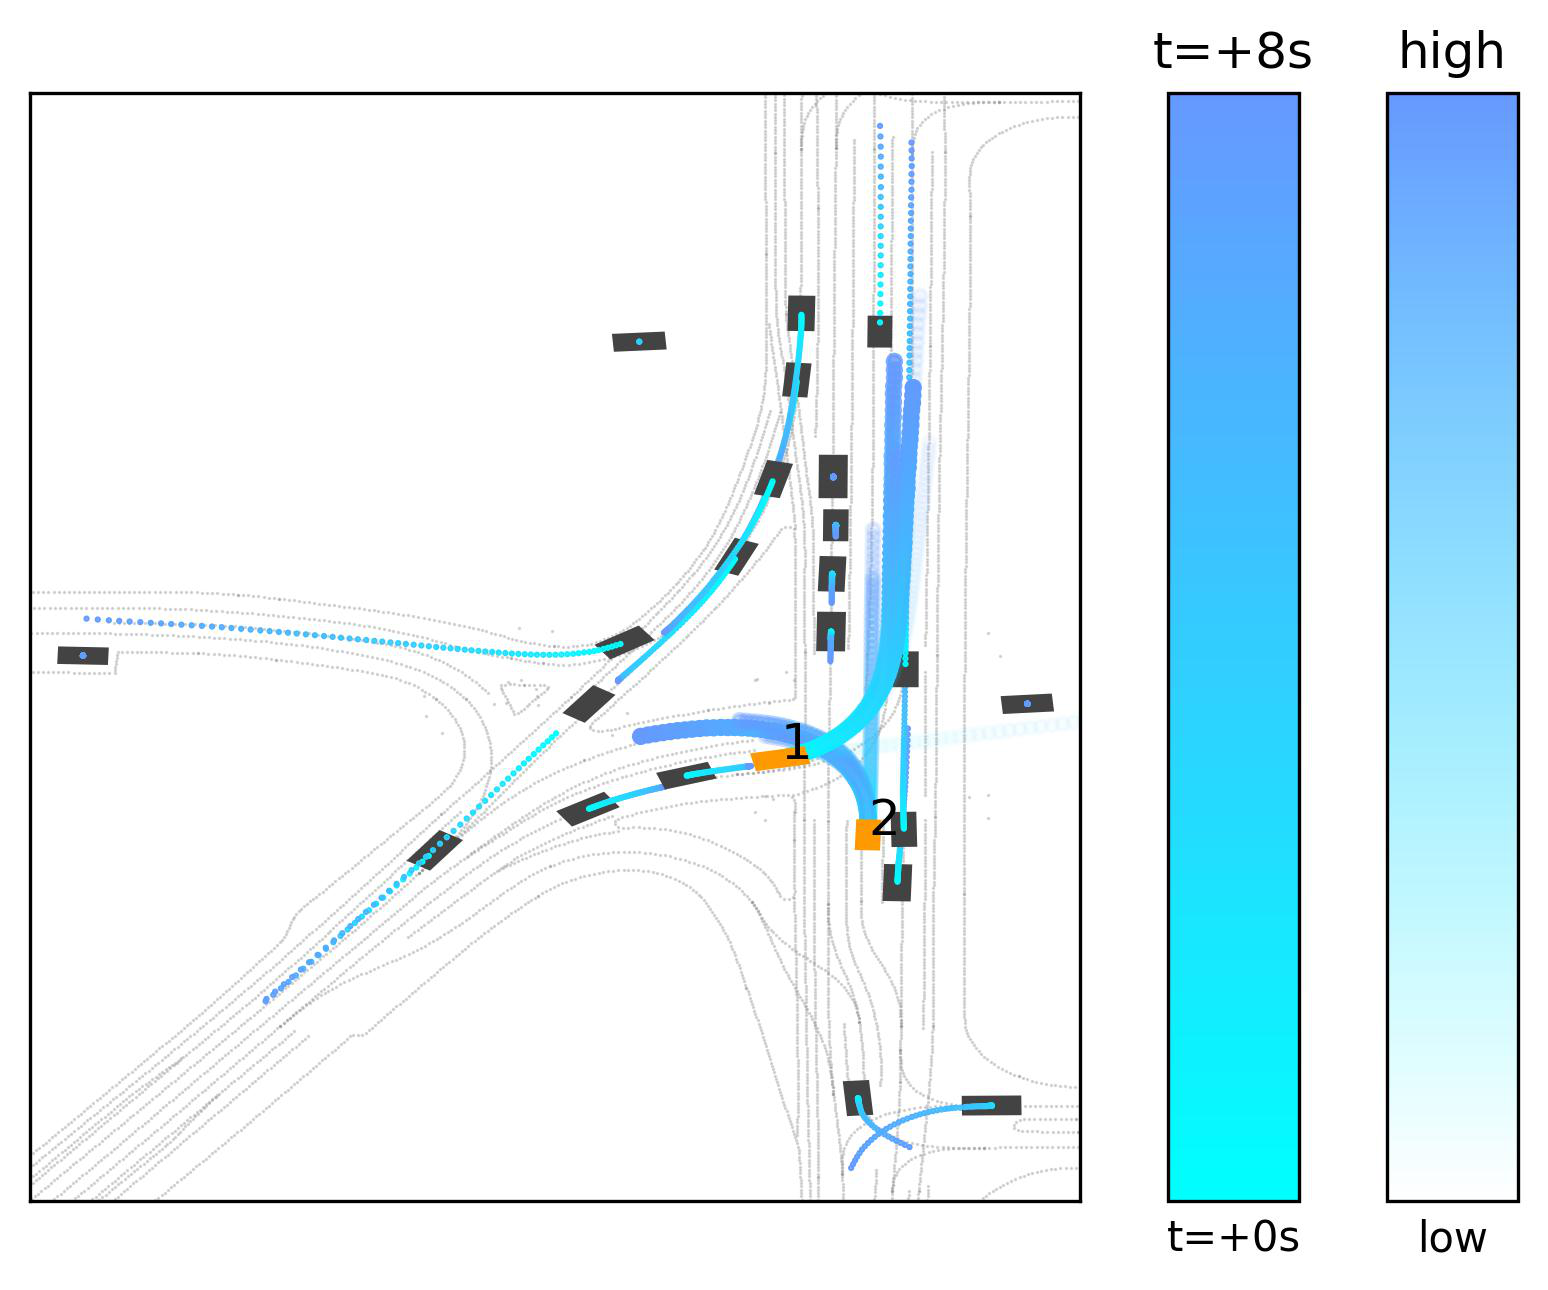}} \\ 
        \subfigure[A cyclist (agent $2$) merges into oncoming traffic. Whether or not they oblige oncoming agent $1$ by using the shoulder affects agent $1$'s speed. ]{\includegraphics[width=0.32\linewidth]{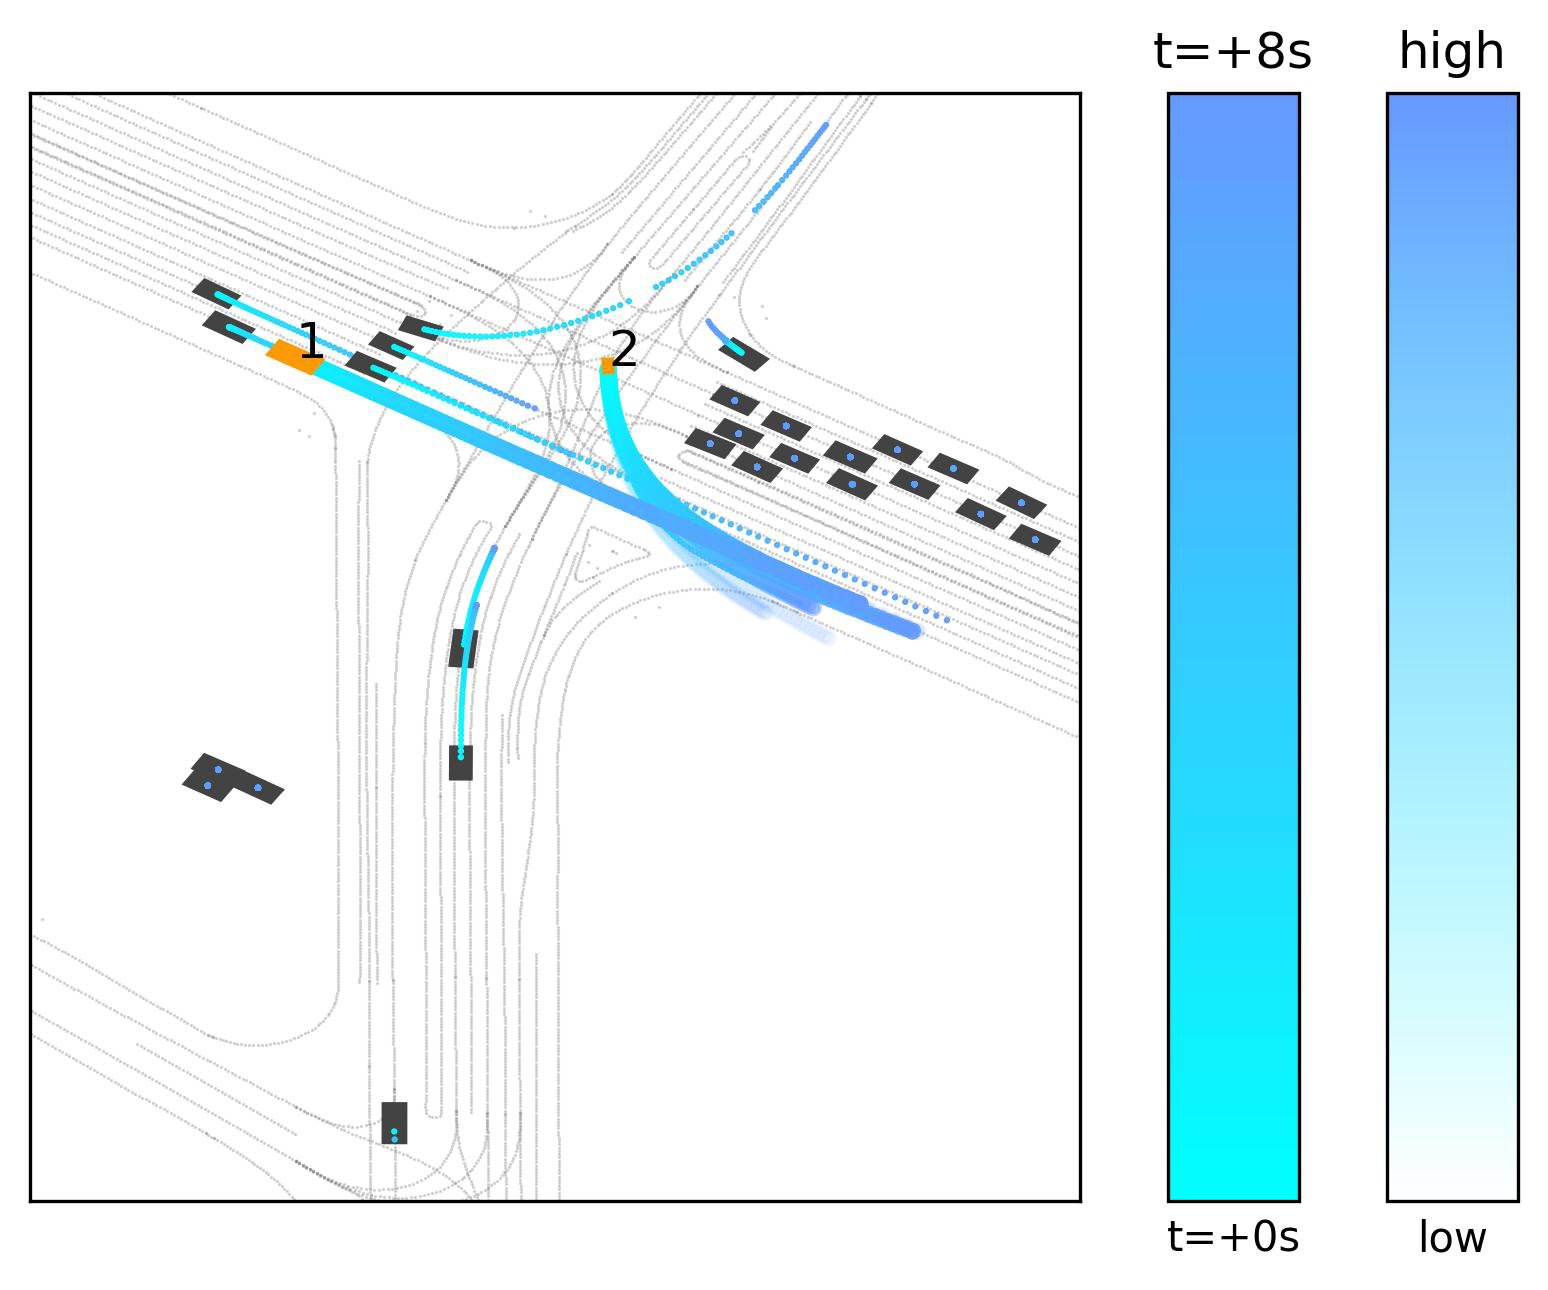}} &
        \subfigure[Turning agent $2$ may accelerate quickly or slowly after the turn ends, affecting agent $1$'s route planning.]{\includegraphics[width=0.32\linewidth]{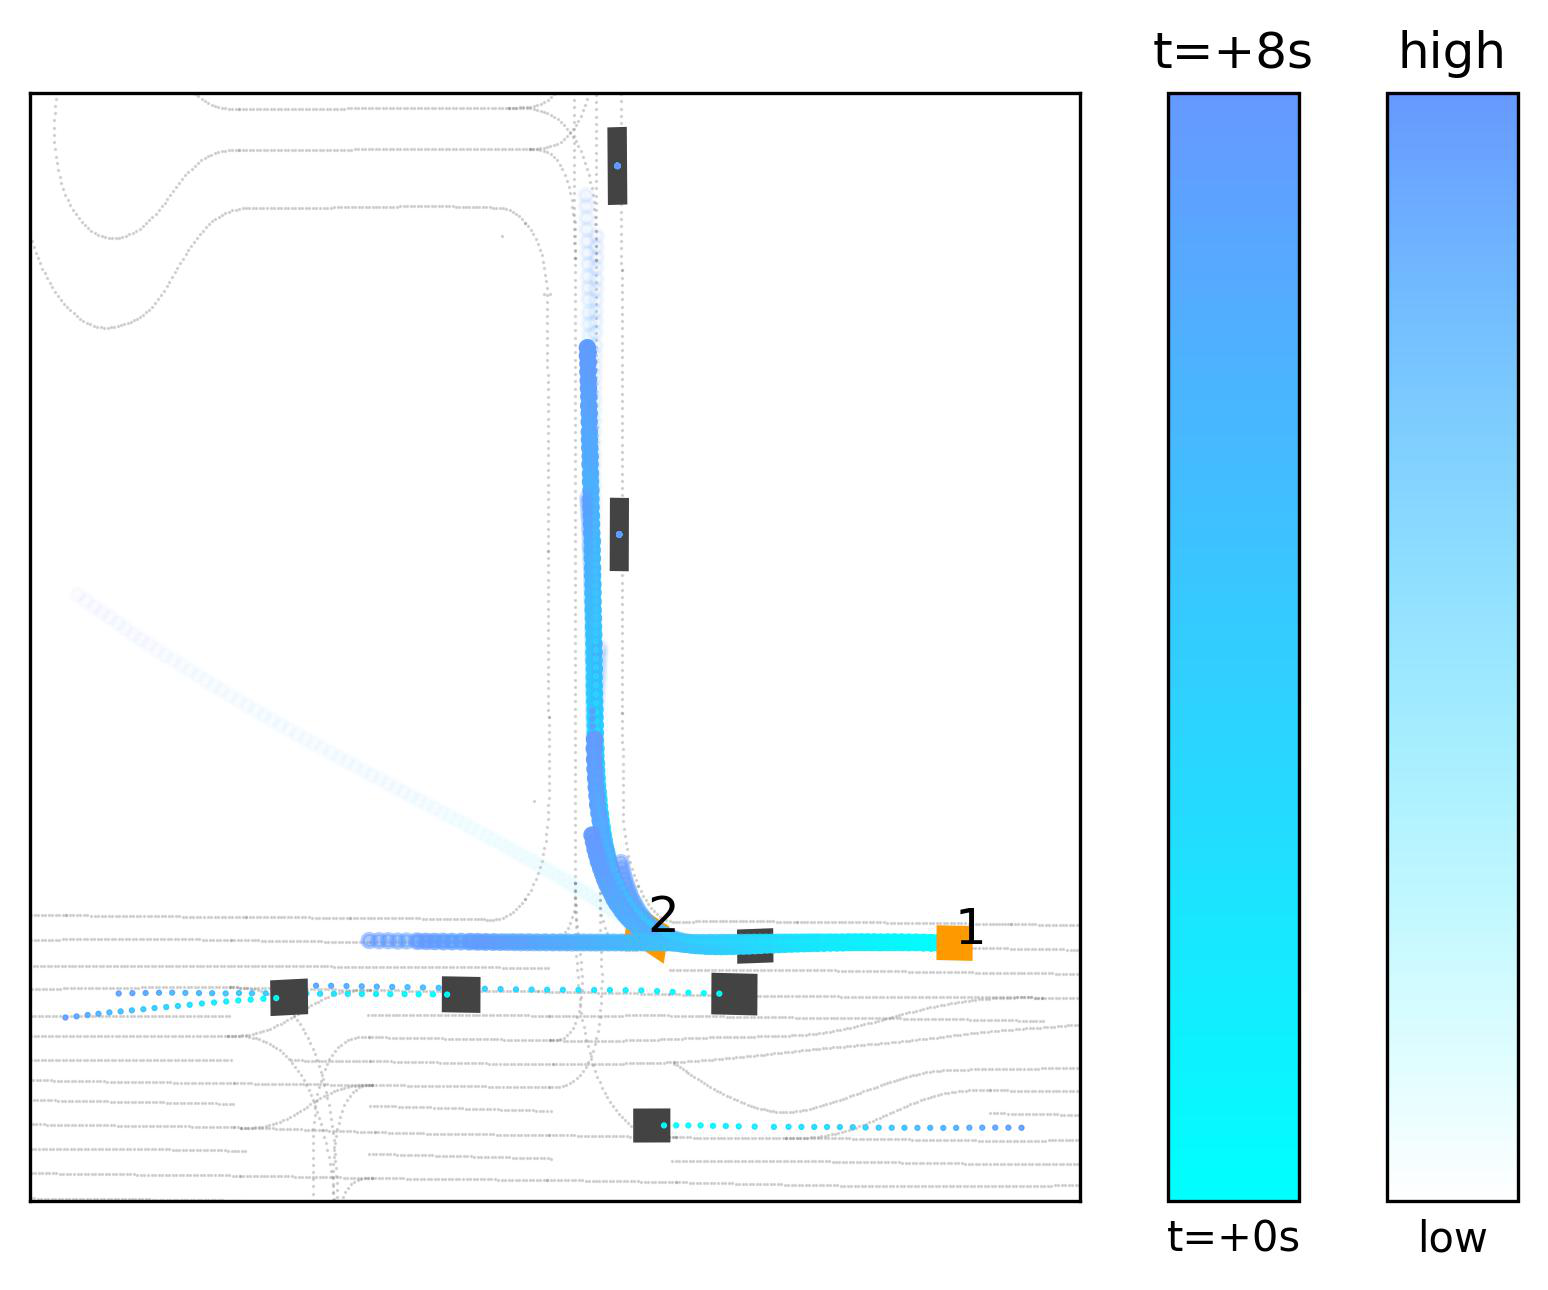}} & 
        \subfigure[Agents $1$ and $2$ both enter a full stop. While agent $2$ has right of way, NashFormer also accounts for the possibility that agent $1$ goes first. ]{\includegraphics[width=0.32\linewidth]{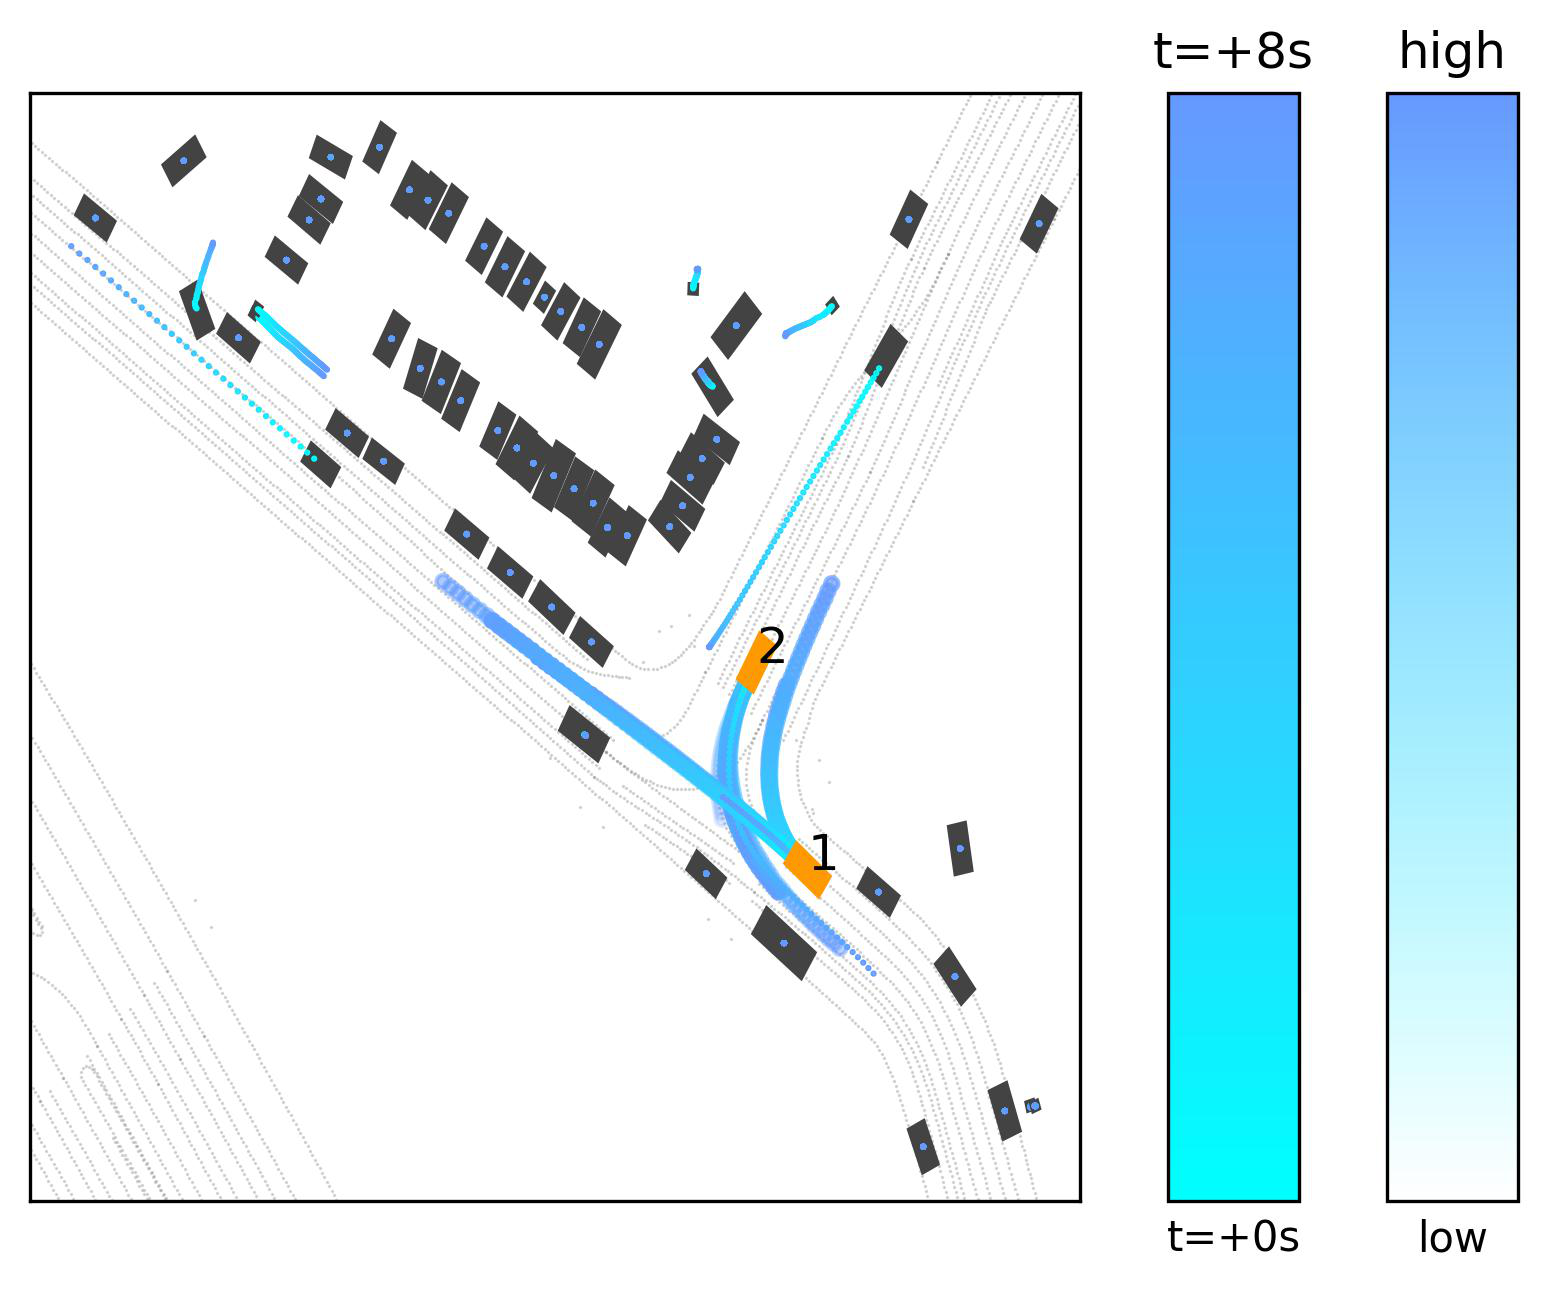}} \\
    \end{tabular}
\caption{Additional qualitative results for NashFormer, exhibiting high coverage of diverse utilities and yield, follow, and close-proximity interactions.}
\label{fig:additional_qualitative}
\end{figure}
