# Supplementary material for: NashFormer: Leveraging Local Nash Equilibria for Semantically Diverse Trajectory Prediction
Source: arXiv:2305.17600 source file (2023-11-11)
Supplement: Supplementary file 2 [file implementation_details.tex]

\subsection{Additional Implementation Details}

\textbf{Marginal Motion Prediction.} We train a single model to predict the joint future motion for three different types of agents: vehicle, pedestrian, and cyclist. Since the number of future agents is bounded at at two, we assign a \textit{joint} motion query for each category combination. The input history state $X$ contains kinematic information for all agents, including position, velocity, acceleration, heading angle, a one-hot vector for the timestamp, and a one-hot vector determining the category of the agent. The input map is pre-processed to include the map point positions, positions of neighboring points, and the heading information of nearby points. Both embeddings have a feature dimension of $256$. For memory-efficient processing, the map is encoded in a lower dimension of $64$ before expansion to dimension $256$. Please refer to \cite{shi2022motion} for additional implementation details.
\\

\textbf{Joint Motion Prediction.} As depicted in Fig.~\ref{fig:predictor_training}, joint motion prediction is obtained via a sort and sum procedure to prioritize the marginal predictions by their individual probabilities. Then, we form the joint prediction by concatenating the $k$ most likely trajectory for each $k$. \textit{Crucially, unlike other approaches \cite{shi2022motion, luo2022jfp}, we retain the gradients for the weights assigned to each marginal mode.} This allows us to differentiate the coverage loss through the sort and sum procedure, resulting in re-weighting of the marginal logits to achieve the correctly weighted joint logits. 
\\

\textbf{Additional Mode Optimization Details.} To find the LNE for each scene, we apply the Mean Shift \cite{cheng1995mean} local optimization algorithm to the trajectories and weights output by the penultimate transformer decoder layer. To stabilize training, we restrict the possible local equilibria only to those points in the prediction set. A bandwidth hyper-parameter controls the radius for local optimization, and the highest-weighted point in each radius is chosen as the local optimization for a fixed iteration. In the next iteration, the local optima of the previous iteration are compared within the same fixed radius. The procedure continues until the number of local optima are stable. We fixed empirically the number of iterations at $10$.  Because the number of equilibira can vary between scenes, the Mean Shift procedure must be performed independently between scenes.
\\

\textbf{Non-Equilibrium Supression (NES)} To prioritize sampling of local Nash equilibria, we propose a procedure similar to non-maximum suppression. Given the set of labels $\boldsymbol{L}$ from the Mean Shift procedure, we iteratively select samples by optimizing the weight within each unique LNE. That is, at iteration $k \in [K]$ of NES, we select $\tau_j$, where $j := \argmax_{i \in L_k} A(\tau_i)$, $L_k$ are the labels associated with the $k$th-highest-weighted LNE, and $j \in [K]$ are the sample indices corresponding to the sorted marginal weights. If one were to perform NMS instead, one would simply take the highest-weighted trajectory within some radius $d$, i.e. $j := \argmax_{\{i: \; ||\tau_i - \tau_k|| < d\}} A(\tau_i)$. Thus, NES functions as NMS with a pairwise equilibrium comparison between samples, rather than a pairwise distance comparison.
\newpage

\begin{figure}[h!]
\centering
\subfigure[Case I: Small threshold fails.]{\includegraphics[width=0.49\textwidth]{img/Sampling/Small Threshold-1.pdf}}
\subfigure[Case II: Large threshold fails.]{\includegraphics[width=0.49\textwidth]{img/Sampling/Large Threshold-3.pdf}}
\caption{Different thresholds for NMS may result in sub-optimal behavior. As a result, the NMS threshold needs to hand-tuned, and the optimal value may very depending on the scenario. In (a), the smaller threshold is too narrow in scope, and NMS chooses sample weights that may belong to the same LNE. In (b), the larger threshold is too broad in scope, and NMS chooses only one LNE, even though there are two distinct local equilibria. Adapted from Figure 4 of \cite{gu2021densetnt}.}
\label{fig:NMS_problem}
\end{figure}

\begin{figure}[h!]
\centering
\settoheight{\tempdima}{\includegraphics[width=.32\linewidth]{img/Sampling/Small Thresh Opt 1-1.pdf}}
\begin{tabular}{@{}c@{ }c@{ }c@{ }c@{}}
&\textbf{Iteration 1} & \textbf{Iteration 2} & \textbf{Iteration 3} \\
\rowname{Case I}& \subfigure[]{\includegraphics[width=0.32\textwidth]{img/Sampling/Small Thresh Opt 1-1.pdf}} & 
\subfigure[]{\includegraphics[width=0.32\textwidth]{img/Sampling/Small Thresh Opt 2-2.pdf}} & 
\subfigure[]{\includegraphics[width=0.32\textwidth]{img/Sampling/Small Thresh Opt 3-2.pdf}} \\
\rowname{Case II} &\subfigure[]{\includegraphics[width=0.32\textwidth]{img/Sampling/Large Threshold Opt 1-3.pdf}} &
\subfigure[]{\includegraphics[width=0.32\textwidth]{img/Sampling/Large Threshold Opt 2-2.pdf}} &
\subfigure[]{\includegraphics[width=0.32\textwidth]{img/Sampling/Large Threshold Opt 3-1.pdf}} 
\label{fig:NES_Small}
\end{tabular}
\caption{Unlike NMS, NES converges to both close-together and far-apart equilibria by using Mean Shift iterates to follow the gradient of the joint density function. All samples that are not equilibia (i.e. not orange stars) are hidden from the sampling until all equilibria have been sampled.}
\end{figure}

% \begin{figure}[h!]
% \centering
% \subfigure[]{\includegraphics[width=0.49\textwidth]{img/Sampling/Too Small Mean Shift-2.pdf}}
% \caption{Although NES prioritizes local equilibria, Mean Shift may erroneously return too few equilibria when the Mean Shift bandwidth is too large, as in Fig.~\ref{fig:NMS_problem}(b), or too many when the bandwidth is too small, as shown here. Unlike Fig.~\ref{fig:NMS_problem}(a), the gradient is noisy and not monotonic. Inspection of the global landscape indicates that there should only be one local maximum. We leave the task of ensuring adequate smoothness in the joint trajectory weights as an area for future work.}
% \label{fig:NMS_problem}
% \end{figure}
% \newpage
