# Supplementary material for: NashFormer: Leveraging Local Nash Equilibria for Semantically Diverse Trajectory Prediction
Source: arXiv:2305.17600 source file (2023-11-11)
Supplement: Supplementary file 3 [file lemma1.tex]

\subsection{Rollout distribution is Boltzmann}

\newtheorem{lemma}{Lemma}
\begin{lemma} (\textnormal{Rollout distribution is Boltzmann})
Let $\mathcal X$ be the space of multi-agent trajectories, and let $\mathcal U$ be the space of admissible controls. Recall that the dynamics satisfy $$x^i = f(x_t, u^1, ..., u^A).$$ Recall that $u^i \sim \pi_\theta(\cdot | x_t) \propto \exp(A_\theta(x,\cdot))$ is the learned game-theoretic policy model. 
Recall from equations \eqref{eqn:log_likelihood} and \eqref{eqn:cumulative_advantage} that the log-probability of a joint trajectory is given as 
\begin{equation}
    \log q_\theta(\tau) = \sum_{t=1}^T \sum_{i=1}^N A^i(x_t, u_t^i) =: A(\tau)
\end{equation}
Then, $q_\theta$ is Boltzmann.
\end{lemma}

\begin{proof}
For any Boltzmann distribution $p$, we have that 
\begin{equation}
    p(\tau) = \exp \big(f(\tau) - \log Z(\tau) \big)
\end{equation}
where $Z(\tau)$ is the partition function. By integrating over $S(\tau)$, we see that  
\begin{equation} \label{lemma1_prod_measure}
    \begin{aligned}
    \log Z(\tau) &= \log   \int_{\mathcal X} \exp A(\tau) d\tau.\\
    &= \log   \int_{\mathcal X} \exp \sum_{t=1}^T \sum_{i=1}^N A^i(x_t, u_t^i) d\tau\\
    &= \log   \int_{\mathcal X}   \prod_{t=1}^T \prod_{i=1}^N \exp A^i(x_t, u_t^i) d\tau\\
    &= \log   \prod_{t=1}^T \prod_{i=1}^N  \int_{\mathcal U}   \exp A^i(x_t, u_t^i) du_t^i\\
    &= \log   \prod_{t=1}^T \prod_{i=1}^N  \int_{\mathcal U}   \exp (Q^i(x_t, u_t^i) - V(x_t)) du_t^i\\
    &= 0.\\
    \end{aligned}
\end{equation}
In the above, the product and integral can be exchanged by Fubini's theorem. The last equality is obtained by definition of the value function.  Therefore, $q_\theta(\tau)$ is Boltzmann with $f(\tau) = A(\tau)$ and $Z(\tau) = 1$.

\end{proof}

\newpage
