# Supplementary material for: NashFormer: Leveraging Local Nash Equilibria for Semantically Diverse Trajectory Prediction
Source: arXiv:2305.17600 source file (2023-11-11)
Supplement: Supplementary file 4 [file lemma2.tex]

\subsection{Equivalence of imitation learning and cross-entropy losses.}

\begin{lemma} (\textnormal{Equivalence of imitation learning and cross-entropy losses.})

Let the space of trajectories $\mathcal X$ and controls $\mathcal U$ be defined as above. Let $p(\tau)$ be the true posterior distribution and $q_\theta$ be the induced posterior distribution under the learned game theoretic policy model, $\pi_\theta \sim \exp(A_\theta(x,a))$. Then, the imitation learning loss \eqref{eqn:dataset_irl_loss} is equivalent to the cross entropy $$H(p, q_\theta) = \int_{\mathcal X} p(\tau) \log q_\theta(\tau) d\tau,$$ up to a constant factor.
\end{lemma}

\begin{proof}
We restate equations \eqref{eqn:item_loss} and \eqref{eqn:dataset_irl_loss} for convenience: 
\begin{equation} \label{eqn:item_loss}
   -\log \pi^i(u|x) = V^i(x) - \bar Q^i(x, u) 
\end{equation}
and
\begin{equation} \label{eqn:dataset_irl_loss}
    \mathcal L_{IRL}(\mathcal D) = -\mathbb E^{\tau \sim \mathcal D}\Bigg[\frac{1}{TA} \sum_{t=1}^T \sum_{i=1}^A \log \pi^i(u|x) \Bigg] .
\end{equation}
Then, for a sufficiently large dataset $\mathcal D$, the imitation learning objective can be expressed (up to a constant factor $TA$) as 
\begin{equation}
    \begin{aligned}
    -TA \cdot \mathcal L_{IRL}(\mathcal D) &= TA \cdot \mathbb E^{\tau \sim p(\tau)}  \big[ \log \pi_{ \theta}^i(u|x_t)] \\
    &= TA \cdot \int_{\mathcal X} p(\tau) \frac{1}{TA} \sum_{t=1}^T \sum_{i=1}^A \big[A_\theta^i(x_t, u_t^i)] d\tau \\
    &= \int_{\mathcal X} p(\tau) \log q_\theta(\tau) d\tau \\
    &= -H(p, q_\theta),
    \end{aligned}
\end{equation}
where we use the definition of the log-probability of the joint trajectory $q_\theta$ from Lemma 1, and where $H$ is the cross entropy between $p$ and $q_\theta$. We approximate the loss $\mathcal L_{IRL}(\mathcal D)$ from a finite sample set as 
\begin{equation}
    \mathcal L_{IRL}(\mathcal D)\approx \frac{1}{S} \sum_{s=1}^S \mathbbm 1_{||\tau_s = \tau|| < \varepsilon} \log q_\theta(\tau_s).
\end{equation}

\end{proof}

\newpage
