# Supplementary material for: NashFormer: Leveraging Local Nash Equilibria for Semantically Diverse Trajectory Prediction
Source: arXiv:2305.17600 source file (2023-11-11)
Supplement: Supplementary file 5 [file nomenclature.tex]

\subsection{Nomenclature}

Table \ref{tab:nomenclature} gives an overview of the symbols and nomencalture presented in this paper. 
\begin{table*}[h!]
    \centering
    \begin{tabular}{l|l}
        \rowcolor{Gainsboro!60} Symbol & Description \\
        \hline \hline
        $A(\cdot)$ & Advantage function\\
        $I$ & Number of gameplay agents \\
        $M$ & Number of distinct LNE, i.e. modes \\
        $N$ & Total number of agents \\
        $L$ & Number of decoder layers \\
        $\boldsymbol L$ & Label set for mode segmentation \\
        $K$ & Number of prediction modes \\
        $T$ & Prediction horizon \\
        $T_0$ & Past horizon \\
        $Q(\cdot)$ & Action-value function \\
        $V(\cdot)$ & Value function \\
        $Z(\cdot)$ & Partition function (same as $V$ in this setting) \\
        $S$ & Final number of samples, after NMS \\
        $b$ & Mean Shift local optimization bandwidth \\
        $f_h^i(\cdot, \cdot)$ & Learnable planar density function\\
        $q$ & Learned distribution of multi-agent trajectories  \\
        $q^*$ & Ideal multi-agent trajectory distribution, after local optimization \\
        $p$ & True distribution of multi-agent trajectories \\
        $\alpha$ & Data loss coefficient \\
        $\beta$ & Classification loss coefficient \\
        $\gamma$ & Coverage loss coefficient \\
        $\theta$ & Learned parameters for the game-theoretic model \\
        $\tau$ & Multi-agent trajectory\\
        $\mathcal U$ & Space of controls, for a single agent \\
        $\mathcal X$ & Space of multi-agent trajectories \\
        $\mathcal S$ & Sample set
    \end{tabular}
    \caption{Nomenclature for NashFormer symbols}
    \label{tab:nomenclature}
\end{table*}
