# Supplementary material for: NashFormer: Leveraging Local Nash Equilibria for Semantically Diverse Trajectory Prediction
Source: arXiv:2305.17600 source file (2023-11-11)
Supplement: Supplementary file 6 [file scenario_details.tex]

\newpage 
\subsection{Measuring Semantic Diversity}

In this section we describe the procedure for measuring semantic diversity, introduced in eqn.~ \eqref{eqn:semantic_coverage}. \\

\paragraph{Filter Descriptions}

We augment the WOMD with semantic labels for the following outcome descriptors: utility, yield, follow, TTC. To measure diversity in the space of utilities, we label the \textit{utility} of an interaction to describe the Boltzmann probability of the final (post-sampling) joint prediction. Since probabilities are continuous, we bin each outcome in $10$ uniform intervals in the range $[0, 1]$. We measure complex network interactions via the \textit{yield} and \textit{follow} labels. An agent \textit{yields} to another if the traces of their trajectories are initially disjoint, they intersect, and then they become disjoint again (e.g. a left turn across an occupied lane).  We bin yields according to the number of yielding agents; the default is $0$, and the maximum is at least $2$. The \textit{follow} label is defined similarly to \textit{yield}, with the only requirement that the traces intersect for at least a second. Finally, to measure close-proximity and coverage of potentially unsafe maneuvers, we measure instances of low time-to-collision (TTC) via a \textit{TTC} label. We bin each \textit{TTC} interaction as described above, according to the number of agents. All of the above filter labels are returned as a one-hot vector indicating the discrete interaction label. The set $\mathcal S$ includes all trajectories with the same one-hot label. The semantic diversity is then computed according to eqn~\eqref{eqn:semantic_coverage}.
\\

\paragraph{Network Interaction Yield Description}

As an auxiliary task, we evaluate NashFormer's ability to cover many LNE in increasingly complex scenarios. We chose to evaluate network \textit{yield} interactions due to the high diversity in potential outcomes when many agents are yielding. For instance, in a four-way stop, the agent that crosses the intersection first will reach its goal before every other agent, but if the same agent becomes must yield, it will be delayed in reaching its goal. Therefore, we construct subsets of the $486$k-example training set of increasingly complex yield interactions by filtering for the \textit{yield} one-hot labels introduced above. We evaluate NashFormer on four different network yield interactions subsets of various size, described in table \ref{tab:yield_table}.
 
\begin{table*}[t!]
    \centering
    \begin{tabular}{l|c}
        \rowcolor{Gainsboro!60} Number of Yields & Count \\
        \hline \hline
        $0$+ & $486$k \\
        $1+$ & $104$k \\
        $2+$ & $21$k \\
        $3+$ & $5$k\\
        $4+$ & $1$k\\
    \end{tabular}
    \caption{Yield interaction subset sizes.}
    \label{tab:yield_table}
\end{table*}
